# Supplementary material for: Green's function retrieval and fluctuations of cross density of states in multiple scattering media
Source: arXiv:1310.5283 source file (2014-01-23)
Supplement: Supplementary file 1 [file supplemental.pdf]

# Supplemental material of "Green's function retrieval and fluctuations of the cross density of states in multiple scattering media"

Julien de Rosny and Matthieu Davy

*Institut Langevin, ESPCI, CNRS, 1 rue Vauquelin, 75231 Paris cedex 05. and Institut d'Electronique et de Télécommunications de Rennes, University of Rennes 1, Rennes 35042, France.*

(Dated: 04/09/2013)

## Abstract

In the first part we show what are the most significant diagrams that contribute to NFC variance and why $\gamma_{2a}$ term dominates when the noise sources are distributed over all the scattering volume. In the second part, we compute the $\gamma_{2a}$ term. Finally we compare the variance of the NCF to the usual intensity fluctuation.

## I. DIAGRAMATIC DEVELOPMENT OF $\left\langle |\zeta|^2 \right\rangle$

As explain in the main article body, the noise cross-correlation function (NCF), it is given by

$$\zeta_S(\mathbf{r}_A, \mathbf{r}_B) \; = \int_V G(\mathbf{r}_A, \mathbf{r}) G^*(\mathbf{r}_B, \mathbf{r}) S(\mathbf{r}) d^3 r. \tag{1}$$

The variance of the NCF is related to the mean square NCF

$$\gamma + |\langle \zeta_S(\mathbf{r}_A, \mathbf{r}_B) \rangle|^2 \; = \left\langle |\zeta_S(\mathbf{r}_A, \mathbf{r}_B)|^2 \right\rangle .$$

From the definition of $\zeta_S$ given by (1), it comes

$$\gamma + |\langle \zeta_S(\mathbf{r}_A, \mathbf{r}_B) \rangle|^2 \; = \int_V \mathscr{G}(\mathbf{r}_A, \mathbf{r}; \mathbf{r}_B, \mathbf{r}') S(\mathbf{r}) S(\mathbf{r}') d^3 r d^3 r'.$$

where

$$\mathscr{G}(\mathbf{r}_\mathrm{A}, \mathbf{r}; \mathbf{r}_\mathrm{B}, \mathbf{r}') \equiv \langle G(\mathbf{r}_A, \mathbf{r}) G^*(\mathbf{r}_B, \mathbf{r}) G(\mathbf{r}_A, \mathbf{r}') G^*(\mathbf{r}_B, \mathbf{r}') \rangle . \tag{2}$$

This term depends on a more general mean value that depends on 8 positions :

$$\langle G(\mathbf{r}_{o1}, \mathbf{r}_{i1}) G^*(\mathbf{r}_{o1'}, \mathbf{r}_{i1'}) G(\mathbf{r}_{o2'}, \mathbf{r}_{i2'}) G^*(\mathbf{r}_{o2}, \mathbf{r}_{i2}) \rangle . \tag{3}$$

On Fig. 1 is shown the diagrammatic representation of the leading terms that contributes to (3) . The development is performed over the number of ladder crossings (i.e., the Hikami constant) up to order 2.

From this expansion, we can deduce the main contributions to $\mathscr{G}(\mathbf{r}_\mathrm{A}, \mathbf{r}; \mathbf{r}_\mathrm{B}, \mathbf{r}')$. They are shown on Fig. (2). Three non-universal fluctuation terms have been added.

In the limit $\|\mathbf{r}_A, \mathbf{r}_B\| \gg \ell_e$, only the diagrams $\gamma_1$, $\gamma_{2a}$ and $\gamma_{3a}$ are significant because the two last scattering of a Ladder are connected to the same position ($\mathbf{r}_A$ or $\mathbf{r}_B$). Diagram $\gamma_1$ is long range in $\mathbf{r}_A$,$\mathbf{r}_B$ but short range in $\mathbf{r}$, $\mathbf{r}'$. Its contribution leads to Gaussian statistics of the NCF and can dominates the other contributions for a small number of noise sources. However, $\gamma_1$ vanishes as soon as the integrations over $\mathbf{r}$ and $\mathbf{r}'$ are performed over a large scattering volume[2]. In that case, the first significant contribution to $\gamma$ is the infinite-range fluctuation $\gamma_{2a}$.

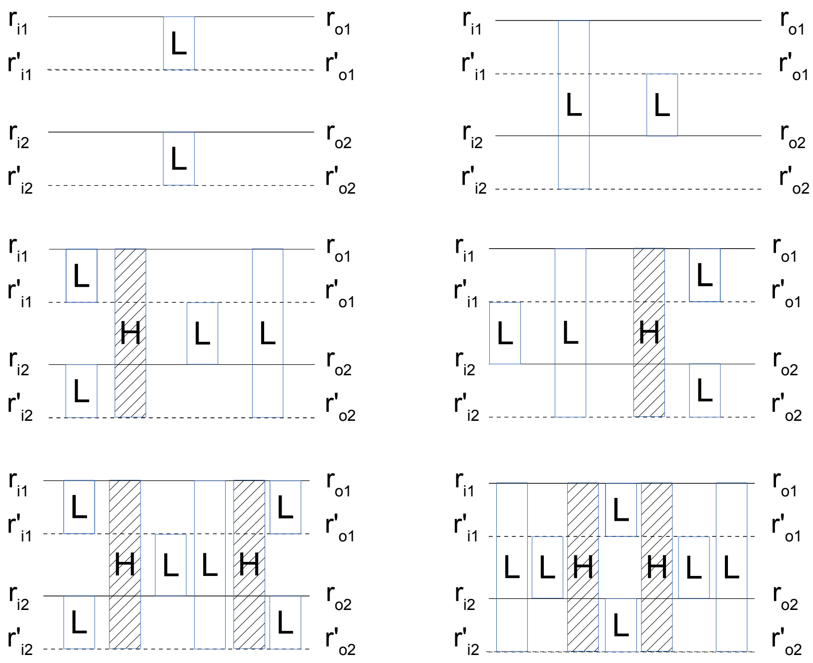


Figure 1: Expansion of $\langle G(\mathbf{r}_{i1}, \mathbf{r}_{o1}) G^*(\mathbf{r}_{i1'}, \mathbf{r}_{o1'}) G(\mathbf{r}_{i2'}, \mathbf{r}_{o2'}) G^*(\mathbf{r}_{i2}, \mathbf{r}_{o2}) \rangle$ up to 2 Hikami vertex.

## II. MATHEMATICAL DERIVATION OF $\gamma$

The variance $\gamma$ of the noise cross-correlation function $\zeta_V$ is given by

$$\begin{aligned} \gamma \;=\; & \int_V \int_V \langle G(\mathbf{r}, \mathbf{r}_A) G^*(\mathbf{r}', \mathbf{r}_A) G^*(\mathbf{r}, \mathbf{r}_B) G(\mathbf{r}', \mathbf{r}_B) \rangle \, d^d\mathbf{r} d^d\mathbf{r}' \\ & - \left| \int_V \langle G(\mathbf{r}, \mathbf{r}_A) G^*(\mathbf{r}', \mathbf{r}_B) \rangle \, d^d\mathbf{r} \right|^2 , \end{aligned}$$

where $d$ is the space dimension . For simplicity, we have replaced $S_V$ by an integration over a finite volume $V$ (which is a surface at 2D).

The mathematical expression of the fluctuation $\gamma_{2a}$ shown in Fig. 2 integrated over $\mathbf{r}$ and $\mathbf{r}'$ is given by

$$\begin{aligned} \gamma_{2a} \;=\; & 2\Delta^4 \Im \langle G(\mathbf{r}_A, \mathbf{r}_A) \rangle \Im \langle G(\mathbf{r}_B, \mathbf{r}_B) \rangle \\ & \times \iiint \Im \langle G(\mathbf{r}, \mathbf{r}) \rangle \Im \langle G(\mathbf{r}', \mathbf{r}') \rangle \, H L(s, r_A) L(s, r_B) L(s, r) L(s, r') d^d r d^d r' d^d s. \end{aligned}$$

Here $H$ is the differential operator of the Hikami vertex. It is given by [3] $H = -h(2\nabla_{r_A}.\nabla_{r_B} + 2\nabla_r.\nabla_{r'} + \nabla_r.\nabla_{r_B} + \nabla_r \nabla_{r_A} + \nabla_r.\nabla_{r_A} + \nabla_r \nabla_{r_B})$, where $h$ is the Hikami

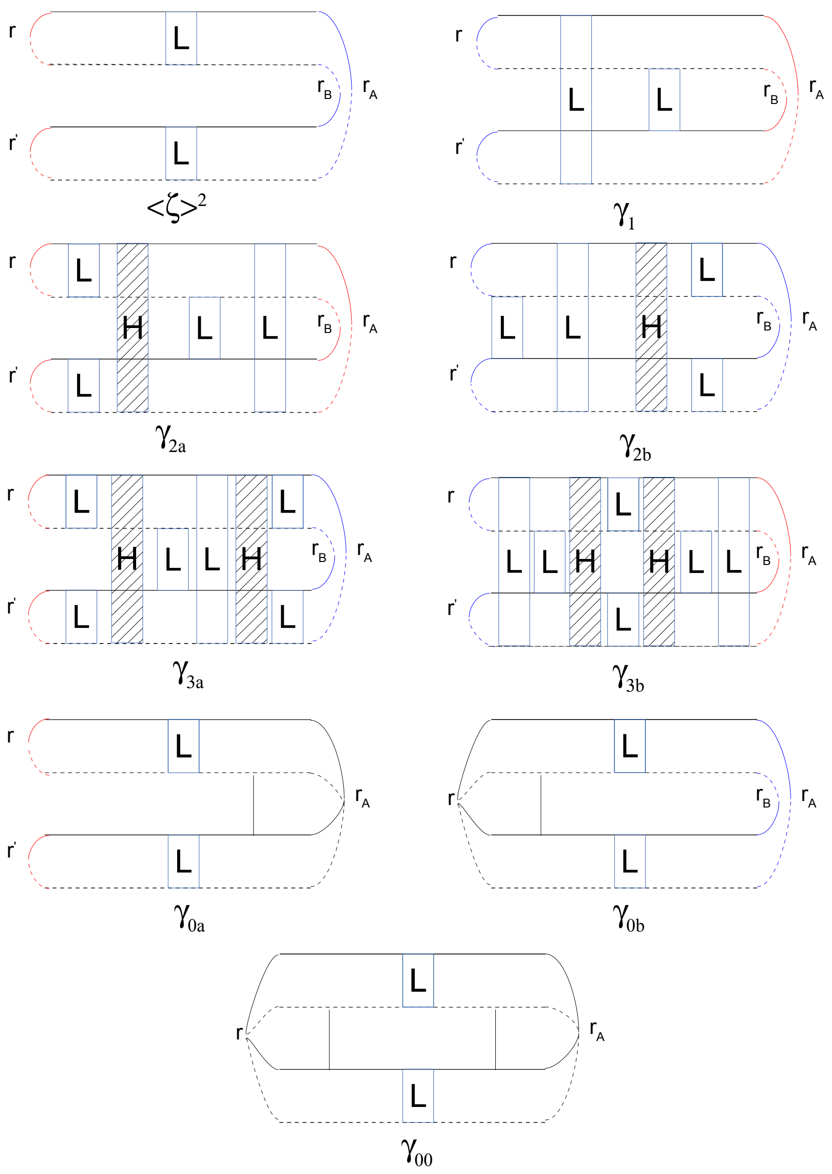


Figure 2: The 6 first diagrams are the most significant contribution to $\mathscr{G}(\mathbf{r}_{\rm A},\mathbf{r};\mathbf{r}_{\rm B},\mathbf{r}')$ up to 2 Hikami vertex. The three last diagrams depends on the details of the local disorder around the probe and involve one or two non-universal vertex [1]. When the last scattering is shown in blue, it implies that the diagrammatic contribution goes toward zeros as soon as the distance between the two positions ($r$,$r'$ or $r_A$, $r_B$) is larger than a mean free path. When the last diffusion is represented in red, the diagrammatic contribution is still significant when the distance between the two positions is larger than a mean free path.

constant and $\Delta = l_e/k$. Six integrals have to be evaluated. Due to the divergence theorem, the five volume integrals that involve $\nabla_r$ or $\nabla_{r'}$ can be expressed as surface integrals, $\int_V \nabla_r L(s,r) d^d r = \int_{A(V)} L(s,r) d^{d-1} r$ , where $A(V)$ is a surface enclosing the volume $V$. Because the medium is slightly lossy, the ladder $L$ falls exponentially with the integration volume so that $\int_{A(V)} L(s,r) d^{d-1} r = 0$. Consequently only the term $\nabla_{r_A}.\nabla_{r_B}$ contributes to $\gamma_{2a}$. It comes

$$\begin{aligned}\gamma_{2a} &= 2h\Delta^4 \iiint \Im \langle G(\mathbf{r},\mathbf{r})\rangle \Im \langle G(\mathbf{r}',\mathbf{r}')\rangle \Im \langle G(\mathbf{r}_A,\mathbf{r}_A)\rangle \Im \langle G(\mathbf{r}_B,\mathbf{r}_B)\rangle \\ &\quad \times L(\mathbf{r},s) L(\mathbf{r}',s) \left[\nabla L(\mathbf{r}_A,s) \nabla L(\mathbf{r}_B,s)\right] d^d r d^d r' d^d s.\end{aligned}$$

The mean value $\Im \langle G(\mathbf{r},\mathbf{r})\rangle$ is a constant equals to $k_0/4\pi$ at 3D and 1/4 at 2D. So the previous expression becomes

$$\gamma_{2a} = 2h\Delta^4 \left(\Im \langle G\rangle \int_V L(\mathbf{r}) d^d r\right)^2 \Im \langle G(\mathbf{r}_A,\mathbf{r}_A)\rangle \Im \langle G(\mathbf{r}_B,\mathbf{r}_B)\rangle \int \nabla L(\mathbf{r}_A,s) \nabla L(\mathbf{r}_B,s) d^d s. \tag{4}$$

The integral $\int_V L(\mathbf{r}) d^d r$ is equal to $K\tau_a$, i.e., $K l_a/c$ where $K$ is source factor of the diffusion equation

$$-D\nabla^2 L(\mathbf{r}_1 - \mathbf{r}_2) + L(\mathbf{r}_1 - \mathbf{r}_2)/\tau_a = K\delta(\mathbf{r}_1 - \mathbf{r}_2).$$

The gradiant product is given by

$$\begin{aligned}2\nabla L(\mathbf{r}_B,s) \nabla L(\mathbf{r}_A,s) &= \nabla[L(\mathbf{r}_A,s) \nabla L(\mathbf{r}_B,s) + L(\mathbf{r}_B,s) \nabla L(\mathbf{r}_A,s)] \\ &\quad - L(\mathbf{r}_A,s) \nabla^2 L(\mathbf{r}_B,s) - L(\mathbf{r}_B,s) \nabla^2 L(\mathbf{r}_A,s).\end{aligned} \tag{5}$$

Because the Ladder L is solution of the diffusion equation, Eq. (5) can be expressed as,

$$\begin{aligned}2\nabla L(\mathbf{r}_A,s) \nabla L(\mathbf{r}_B,s) &= -L(\mathbf{r}_A,s) \left[\frac{1}{D\tau_A} L(\mathbf{r}_B,s) - \frac{K}{D}\delta(\mathbf{r}_B - s)\right] \\ &\quad - L(\mathbf{r}_B,s) \left[\frac{1}{D\tau_A} L(\mathbf{r}_A,s) - \frac{K}{D}\delta(\mathbf{r}_A - s)\right].\end{aligned}$$

The integration over volume V leads to

$$2\int_V \nabla L(\mathbf{r}_A,s)\nabla L(\mathbf{r}_B,s)d^ds \;=\; \frac{K}{D}\left[L(\mathbf{r}_A,\mathbf{r}_B)+L(\mathbf{r}_B,\mathbf{r}_A)\right].$$

because at 3D$\frac{1}{\tau_a}\int_V L(\mathbf{r}_A,s)L(\mathbf{r}_B,s)d^ds < \frac{1}{\tau_a}\int_V L^2(\mathbf{r}_A,s)d^3s \sim \frac{K^2}{D^2\tau_a}\sqrt{D\tau_a}$. So when $\tau_A \to \infty$, the integral goes toward 0. At 2D, the demonstration is much more difficult because $\int L^2(\mathbf{r}_A,s)d^2s$ scales as $\tau_A$ but the result is identical.

The reciprocal property of the diffusion, i.e., $L(\mathbf{r}_A,\mathbf{r}_B)=L(\mathbf{r}_B,\mathbf{r}_A)$ leads to

$$\int_V \nabla L(\mathbf{r}_A,s)\nabla L(\mathbf{r}_B,s)d^ds \;=\; \frac{K}{D}L(\mathbf{r}_A,\mathbf{r}_B).$$

It finally comes the expression presented in the main article.

$$\gamma_{2a} = 2h\Delta^4\left(\Im\langle G\rangle\int_V L(\mathbf{r})d^dr\right)^2 \Im\langle G(\mathbf{r}_A,\mathbf{r}_A)\rangle\,\Im\langle G(\mathbf{r}_B,\mathbf{r}_B)\rangle\,\frac{K}{D}L(\mathbf{r}_A,\mathbf{r}_B). \tag{6}$$

## III. SYSTEMATIC COMPARISON BETWEEN INTENSITY AND CROSS-CORRELATIONS FLUCTUATIONS

The aim of part is to systematically compare intensity and the cross-correlations functions (CCF) fluctuations and to show that they are not identical.

In a similar way to $\zeta_S$, we introduce the intensity produced at position $\mathbf{r}_A$ by a distribution of uncorrelated sources. The intensity for a single realization of disorder is then given by

$$I_S(\mathbf{r}_A) \;=\; \int_V G(\mathbf{r}_A,\mathbf{r})G^*(\mathbf{r}_A,\mathbf{r})S(\mathbf{r})d^3r,$$

where S is the power spectrum source distribution. The mean intensity is therefore

$$\langle I_S(\mathbf{r}_A)\rangle \;=\int_V\; \langle G(\mathbf{r}_A,\mathbf{r})G^*(\mathbf{r}_A,\mathbf{r})\rangle\, S(\mathbf{r})d^3r_S.$$

Now we estimate the intensity correlation between the intensity recorded at position A and position B for two identical noise source distributions :

$$\begin{aligned} C_I \;&\equiv\; \langle I_S(\mathbf{r}_A)I_S(\mathbf{r}_B)\rangle \\ &=\; \int_V \mathscr{C}(\mathbf{r}_A,\mathbf{r};\mathbf{r}_B,\mathbf{r}')S(\mathbf{r})S(\mathbf{r}')dr^3dr^3. \end{aligned}$$

where

$$\mathscr{C}(\mathbf{r}_\mathrm{A},\mathbf{r};\mathbf{r}_\mathrm{B},\mathbf{r}') \equiv \langle G(\mathbf{r}_A,\mathbf{r}_S)G^*(\mathbf{r}_A,\mathbf{r}_S)G(\mathbf{r}_B,\mathbf{r}_{S'})G^*(\mathbf{r}_B,\mathbf{r}_{S'})\rangle \,. \tag{7}$$

Thus, as for $\mathscr{G}$, $\mathscr{C}$ can be deduced from the general expression $\langle G(\mathbf{r}_{o1},\mathbf{r}_{i1})G^*(\mathbf{r}_{o1'},\mathbf{r}_{i1'})G(\mathbf{r}_{o2'},\mathbf{r}_{i2'})G^*(\mathbf{r}_{o2},\mathbf{r}_{i2})\rangle$. On Fig. 3, we have drawn the major contributions to $\mathscr{C}$.

Note that difference between $\mathscr{C}$ and $\mathscr{G}$ resides in a single position permutation on the right hand side of the diagrams. This permutation induces that NCF contributions cannot directly deduced from the intensity ones when $\mathbf{r}_A \neq \mathbf{r}_B$ even after integration over $\mathbf{r}$ and $\mathbf{r}'$. Functions $\mathscr{G}$, $\mathscr{C}$ becomes equal when $\mathbf{r}_A = \mathbf{r}_B$. In this last case, the contribution to NCF fluctuations and intensity correlations are identical.

To conclude, we see on this systematic comparison between the intensity and NCF fluctuations that both of them are based on a same expansion of the mean value of the product of four Green's functions (depicted on Fig. 1). But because of a single position permutation the properties between intensity correlation and NCF fluctuations are different. This difference is very important and is the origin of the results shown in the paper.

---


[1] B. Shapiro, Phys. Rev. Lett. **83**, 4733 (1999), `http://link.aps.org/doi/10.1103/PhysRevLett.83.4733`.

[2] B. Van Tiggelen and S. Skipetrov, Phys. Rev. E **73**, 045601 (2006), `http://pre.aps.org/abstract/PRE/v73/i4/e045601`.

[3] R. Berkovits and S. Feng, Phys. Rep. **238**, 135 (1994), `http://www.sciencedirect.com/science/article/pii/0370157394900795`.

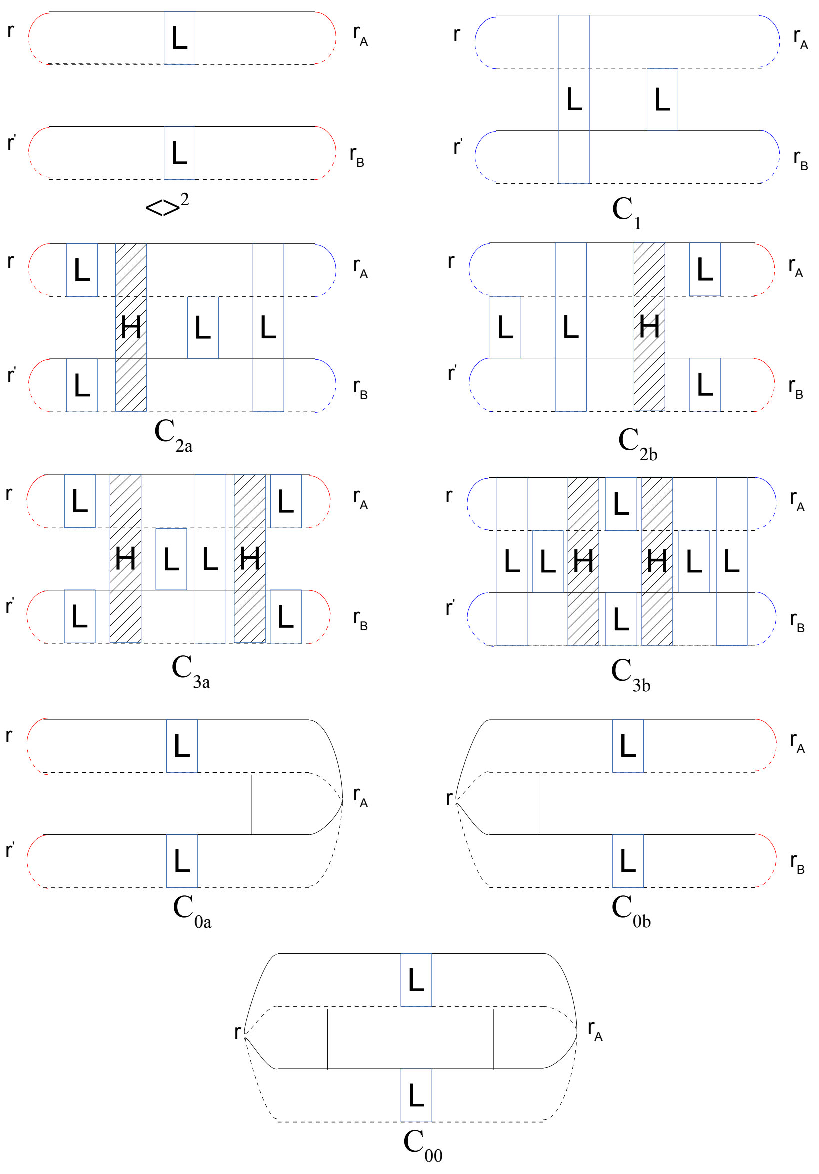


Figure 3: The 6 first diagrams are the leading terms of $\mathscr{C}(\mathbf{r}_{\mathrm{A}}, \mathbf{r}; \mathbf{r}_{\mathrm{B}}, \mathbf{r}')$ up to 2 Hikami vertex. The three last diagrams involved near probe scattering correlations. When the last scattering is shown in blue, it implies that the diagrammatic contribution goes toward zeros as soon as the distance between the two positions ($\mathbf{r}$,$\mathbf{r}'$ or $\mathbf{r}$, $\mathbf{r}_B$) is larger than a mean free path. When the last diffusion is represented in red, the diagrammatic contribution is still significant when the distance between the two positions is larger than a mean free path.
